# Supplementary material for: Reliable Physiological Monitoring on the Wrist Using Generative Deep Learning to Address Poor Skin-Sensor Contact
Source: arXiv:2504.02735 source file (2025-04-16)
Supplement: Supplementary file 1 [file Appendix.tex]

\clearpage 
\section*{Appendix}
